# Supplementary material for: Materials properties of out-of-plane heterostructures of MoS$_2$-WSe$_2$ and WS$_2$-MoSe$_2$
Source: arXiv:1602.00028 source file (2016-01-29)
Supplement: Supplementary file 1 [file supplementary.tex]

\documentclass[10pt,aps,preprint,pra,twocolumn]{revtex4}

\usepackage{graphicx}

\usepackage{multirow}

\begin{document}

\title{Materials properties of out-of-plane heterostructures of MoS$_2$-WSe$_2$ and WS$_2$-MoSe$_2$}
\author{Bin Amin}
%\email{binukhn@gmail.com, +92-333-943-4665}
\affiliation{Department of Physics, Hazara University, Mansehra, Karakoram Hwy, Dhodial 21120, Pakistan}
\author{Thaneshwor P. Kaloni} 
%\email{thaneshwor.kaloni@umanitoba.ca,+1-204-952-2900}
\affiliation{Department of Chemistry, University of Manitoba, Winnipeg, Manitoba R3T 2N2, Canada}
\author{Georg Schreckenbach}
\affiliation{Department of Chemistry, University of Manitoba, Winnipeg, Manitoba R3T 2N2, Canada}
\author{Michael S. Freund}
\affiliation{Department of Chemistry, University of Manitoba, Winnipeg, Manitoba R3T 2N2, Canada}
\maketitle

\section{Computational detail}

Density functional theory with the Perdew-Burke-Ernzerhof (PBE) \cite{Perdew96} and Heyd-Scuseria-Ernzerhof (HSE06) functionals \cite{Heyd} implemented in the VASP package were used.\cite{Kresse93}. The Van der Waals interactions (Grimme's approach) were taken into account to optimize the geometries as well as to perform further calculations.\cite{Grimme} A vacuum layer of 18 \AA\ is used to prevent artifacts due to the periodic boundary conditions. The structures were optimized until the forces and energy reached to 0.0001 eV/\AA\ with a high plane wave cutoff of 700 eV. A $6\times6\times1$ k-mesh was used for the optimizations. It was further refined to a $12\times12\times1$ mesh for the subsequent calculation of the electronic and vibrational properties. Relativistic effects including spin-orbit coupling are significant for the heavy elements (Mo and W) and hence, spin-orbit and relativistic pseudopotentials have been using in the calculations. In order to study the optical spectrum, the quasi-particle self-energy corrections (GW$_0$) approach has been used to solve the Bethe-Salpeter equation (Tamm-Dancoff approximation).\cite{Agisilaos13} The 10 highest valence and 10 lowest conduction bands were taken into account in calculating the excitonic eigenstates.

\end{document}
